# Supplementary material for: Assessing the Resilience of Automotive Intrusion Detection Systems to Adversarial Manipulation
Source: arXiv:2506.10620 source file (2025-06-12)
Supplement: Supplementary file 1 [file appendix.tex]

\section{Overflow form other sections}
\label{sec:set-diff-dodis}
Sometime you ware super excited about some details that does not quite fit with
the rest of the paper goes here. For example, some details about how you
instrumented the Android Linux kernel should go to appendix, and for really
curious reader to read. Remember it's appendix, so the reader is not required to
read, and you should not put critical information in appendix that is crucial
for understanding the rest of the paper.

%%% Local Variables:
%%% mode: latex
%%% TeX-master: "main"
%%% End:
